# Supplementary material for: Enhancing Energy-Awareness in Deep Learning through Fine-Grained Energy Measurement
Source: arXiv:2308.12264 source file (2024-02-01)
Supplement: Supplementary file 1 [file total_energy_df.tex]

\begin{tabular}{llrrrrrrr}
 & function & run time & CPU (mean) & CPU (median) & RAM (mean) & RAM (median) & GPU (mean) & GPU (median) \\
0 & tensorflow.keras.models.Sequential.fit & 168.96 & 2038.00 & 2037.97 & -8.94 & -9.84 & 8474.62 & 7609.72 \\
1 & tensorflow.keras.models.Sequential.evaluate & 1.90 & 14.49 & 14.83 & 0.81 & 0.83 & 38.99 & 45.80 \\
2 & method-level (sum) & 170.85 & 2052.49 & 2052.80 & -8.13 & -9.01 & 8513.61 & 7655.52 \\
3 & project-level & 174.32 & 2189.51 & 2160.96 & 30.44 & 28.43 & 10314.85 & 10347.04 \\
\end{tabular}
